# Supplementary material for: Data-Driven Stochastic Modeling of Schooling Fish: From Collective Dynamics to Individual Fluctuations
Source: arXiv:2509.08630 ancillary file (2026-01-14)
Supplement: Supplementary file 1 [file Stochastic_modelling_of_fish_shooling_dynamics_SM.pdf]

# Stochastic Modeling of Fish Schooling Dynamics: Decomposition into Collective and Individual Movements

## Supplemental Material

Elena G. de Lamo,<sup>1</sup> M. Carmen Miguel,<sup>2,3</sup> and Romualdo Pastor-Satorras<sup>1</sup>

<sup>1</sup>*Departament de Física, Universitat Politècnica de Catalunya, Campus Nord B4, 08034 Barcelona, Spain*

<sup>2</sup>*Departament de Física de la Matèria Condensada,*

*Universitat de Barcelona, Martí i Franquès 1, 08028 Barcelona, Spain*

<sup>3</sup>*Institute of Complex Systems (UBICS), Universitat de Barcelona, 08028 Barcelona, Spain*

### SM-I. EXPERIMENTAL DATA COLLECTION

Experiments were conducted at the Scientific and Technological Centers UB (CCiTUB), University of Barcelona (Spain), and were reviewed and approved by the Ethics Committee of the University of Barcelona (project number 119/18). We used schooling fish of the species *Hyphessobrycon herbertaxelrodi* (black neon tetra), a small freshwater species with an average body length of approximately 2.5cm, known for forming coherent, highly polarized, and planar schools [1]. The experiments involved schools of  $N = 40, 50$  and 60 individuals swimming freely in a experimental tank of dimensions  $100 \times 100 \times 40$  cm, with a water column height of 7 cm. Due to this species' tendency to swim close to the water surface, the fish movement was effectively two-dimensional.

Fish were recorded with a GoPro Hero 11 Black camera at 50 fps and a resolution of  $5312 \times 2988$  pixels, mounted 1 m directly above the tank. The side length of the tank in the recordings corresponded to  $L = 2730$  pixels, which was used as a scale to recover physical dimensions from the video data. For each group size, three independent 60-minute recordings were made (totaling 180,000 frames per recording).

Individual fish trajectories were extracted by digitizing the videos using the open-source software `idtracker.ai` [2]. Occlusions causing invalid position data were corrected with the Validator tool included in version 5 of `idtracker.ai`. To reduce noise, trajectories were smoothed with a Gaussian filter [3] with  $\sigma = 5$ , truncating the filter at  $5\sigma$ , using the `scipy.ndimage.gaussian_filter1d` function from the SciPy library [4]. Individual velocities and accelerations were obtained by differentiating the smoothed trajectories using the first and second derivatives of the Gaussian kernel, respectively.

### SM-II. PARAMETER OPTIMIZATION OF THE CM DYNAMICS

The characteristic speed  $V_0$  was independently estimated from the experimental velocity distributions. Specifically, we fitted a Gaussian mixture model to the empirical distributions  $P(V_x, 0)$  and  $P(0, V_y)$ , (see Fig. SF1). The distributions were constructed by aggregating data points within a small interval  $[-\Delta V_i, \Delta V_i]$ , where  $\Delta V_i = 0.6\text{cm/s}$  was chosen to balance statistical significance and resolution. To ensure consistency and symmetry, we verified that the estimated values of  $V_0$  were symmetric around zero, passing a skewness test with a  $p$ -value greater than 0.05. The final value of  $V_0$  was obtained by averaging the absolute values of the means derived from the individual Gaussian fits to each profile of the joint distribution.

The average radius of gyration is computed as

$$R_g = \left\langle \sqrt{\sum_i [\vec{r}_i(t)]^2 / N} \right\rangle_t \quad (\text{SE1})$$

where the average is taken over all experimental frames for each system size  $N$ .

To optimize the remaining parameters  $\gamma$ ,  $U_0$ ,  $\ell$ ,  $a$ , and  $D$  of the model, we minimized the symmetric Kullback–Leibler (KL) divergence between the probability density functions (PDFs) of position and velocity obtained from numerical simulations and those measured experimentally [5]. The KL divergence between two distributions  $P$  and  $Q$  is defined as

$$D_{KL}(P, Q) = \sum_i P(i) \ln \frac{P(i)}{Q(i)}. \quad (\text{SE2})$$

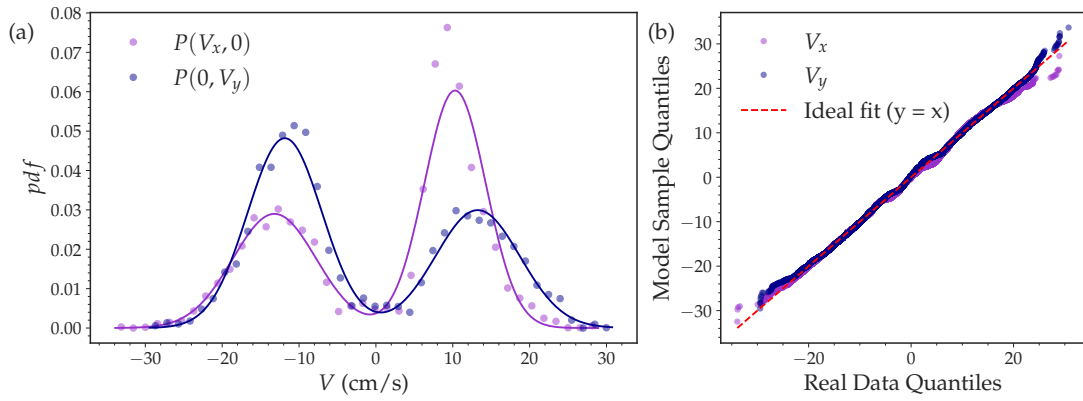

Figure SF1: Gaussian mixture modeling of the center-of-mass (CM) velocity. (a) The empirical distribution is well described by a Gaussian mixture. (b) A Q-Q plot corroborates the quality of the fit. The Kolmogorov–Smirnov test produces  $p$ -values of 0.06 for the  $v_x$  component and 0.34 for the  $v_y$  component, indicating no significant deviation from the modeled distribution.

|      | $U_0$ [cm/s <sup>2</sup> ] | $a$             | $\gamma_0$ [s <sup>-1</sup> ] | $\ell$ [cm]    | $\sqrt{2D}$ [cm s <sup>-3/2</sup> ] | $R_g$ [cm]         | $V_0$ [cm/s]   |
|------|----------------------------|-----------------|-------------------------------|----------------|-------------------------------------|--------------------|----------------|
| N=40 | 21.38                      | 0.82            | 1.17                          | 13.60          | 7.50                                | $17.083 \pm 0.007$ | $11.6 \pm 0.4$ |
|      | 22.38                      | 0.72            | 0.92                          | 19.36          | 7.12                                | $18.063 \pm 0.006$ |                |
|      | $21.9 \pm 0.4$             | $0.77 \pm 0.04$ | $1.01 \pm 0.09$               | $16 \pm 2$     | $7.3 \pm 0.2$                       | $17.8 \pm 0.3$     |                |
| N=50 | 17.38                      | 0.94            | 0.98                          | 19.08          | 6.55                                | $16.024 \pm 0.008$ | $12.1 \pm 0.7$ |
|      | 14.76                      | 0.88            | 1.46                          | 15.02          | 7.52                                | $18.89 \pm 0.01$   |                |
|      | 22.84                      | 0.69            | 1.00                          | 17.95          | 7.44                                | $19.16 \pm 0.01$   |                |
|      | $18 \pm 2$                 | $0.84 \pm 0.06$ | $1.1 \pm 0.2$                 | $17 \pm 1$     | $7.2 \pm 0.5$                       | $18.0 \pm 0.8$     |                |
| N=60 | 21.48                      | 0.70            | 1.28                          | 16.21          | 6.26                                | $23.17 \pm 0.01$   | $11.6 \pm 0.5$ |
|      | 17.81                      | 0.79            | 1.57                          | 16.95          | 6.20                                | $23.49 \pm 0.01$   |                |
|      | 18.32                      | 0.78            | 1.66                          | 16.84          | 5.69                                | $24.184 \pm 0.007$ |                |
|      | $19 \pm 1$                 | $0.76 \pm 0.03$ | $1.5 \pm 0.1$                 | $16.7 \pm 0.2$ | $6.0 \pm 0.2$                       | $23.6 \pm 0.3$     |                |

Table ST1: Optimal parameter sets, obtained by minimizing the KL divergence across different experiments, are reported alongside the value of  $V_0$  derived from Gaussian fitting. The final row for each group size  $N$  represents the mean of the three optimized results, with uncertainties corresponding to the standard error of the mean. The results are organized according to the number of fish in the school. For  $N = 40$ , only two experimental solutions are available instead of three, as the KL divergence in one experiment converged to a non-physical solution ( $a < 0$ ).

In our case, the objective function to be minimized is the sum of the symmetric KL divergences for both the position and velocity distributions:

$$D_{KL}^{tot} = D_{KL}^{pos}(P, Q) + D_{KL}^{pos}(Q, P) + D_{KL}^{vel}(P, Q) + D_{KL}^{vel}(Q, P),$$

where  $P$  denotes the experimental distributions and  $Q$  the simulated distributions given the model parameters  $\{\gamma_0, a, U_0, \ell, \sqrt{2D}\}$ . To identify the optimal parameters, we repeated the KL divergence minimization across different random seeds and computed the average of the resulting KL divergence values. This approach helps mitigate the effects of variability inherent to individual simulation runs. Additionally, the optimization was performed starting from multiple initial conditions to ensure convergence to the global minimum.

The parameters resulting from this optimization are listed in Table ST1. Regarding their dependence on the number of individuals  $N$ , the friction coefficient  $\gamma_0$  increases as  $N$  grows, while the noise amplitude  $\sqrt{2D}$  decreases markedly as  $N$  grows. The remaining parameters show no clear dependence on  $N$ .

Fig. SF2 shows the relationship between the computed friction coefficient  $\gamma_0$  and the experimentally measured radius of gyration  $R_g$ . The results indicate a roughly linear trend between these parameters, although the correlation is moderate, with an  $r^2$  value of approximately 0.6.

Our findings suggest that the center-of-mass dynamics of fish schools qualitatively resemble those of an inertial active Brownian particle experiencing hydrodynamic drag. The measured  $\gamma_0$  value reflects the system's intrinsic variability, which is expected given that fish schools are deformable structures composed of individually active agents.

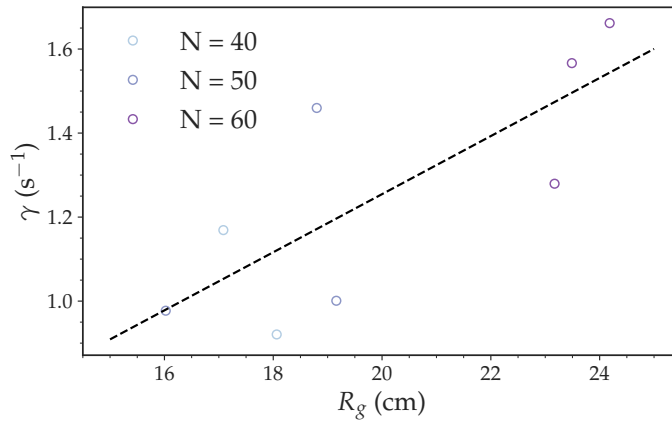

Figure SF2: Relation between the fiction coefficient  $\gamma_0$ , computed through KL divergence minimization for each experiment, and average  $R_g$  computed experimentally. Value of the coefficient of determination  $r^2 = 0.591$ .

### SM-III. NON-LINEAR FIT TO THE RADIAL PARTICLE DENSITY

The empirical radial particle density in the CM reference frame (Fig. 2(b) in the main paper) was fitted to the functional form

$$\rho(r) = \frac{a}{b + e^{ar}}. \quad (\text{SE3})$$

Non-linear fitting was performed using the `scipy.optimize.curve_fit` function from the `Scipy` Python scientific library [4]. The resulting parameters are reported in Table ST2. From here, the effective force in Cartesian coordinates,  $f_{\text{eff}}(r)$ , can be derived from Eq. (5) in the main paper.

These parameters provide insights into the effective interaction forces that confine individual fish within the school. For small distances  $r < R_g$ , the denominator is dominated by the constant term  $b \gg e^{ar}$ , since  $a \propto 1/R_g$  (Fig. SF3). This results in an approximately uniform density  $\rho = a/b$ , and the effective radial force simplifies to  $f_{\text{eff}}(r) \approx \frac{a}{b+1} \approx 0$ , given that  $b \gg a$ . As  $r$  exceeds  $R_g$ , the exponential term becomes significant, leading to a gradual decline in  $\rho(r)$  and causing  $f_{\text{eff}}(r)$  to approach a gentle, nearly constant restoring force. This suggests that fish experience minimal confinement within the group but are gently pulled back when they venture beyond its boundary. A plausible explanation is that vision—likely the primary sensory modality driving schooling behavior at length scales beyond immediate proximity [6]—enables fish to feel secure as long as they maintain visual contact with conspecifics. Only when they venture too far away do they respond as if subjected to a pulling force aimed at restoring group cohesion. However, as long as fish retain visual contact, they experience a relatively constant pulling force regardless of their distance from the group center.

| $N$ | $a$               | $b$          | $\alpha[\text{cm}^{-1}]$ |
|-----|-------------------|--------------|--------------------------|
| 40  | $0.34 \pm 0.02$   | $466 \pm 18$ | $0.313 \pm 0.002$        |
|     | $0.258 \pm 0.006$ | $406 \pm 10$ | $0.282 \pm 0.001$        |
|     | $0.28 \pm 0.01$   | $437 \pm 16$ | $0.291 \pm 0.002$        |
| 50  | $0.301 \pm 0.006$ | $354 \pm 8$  | $0.321 \pm 0.001$        |
|     | $0.062 \pm 0.003$ | $84 \pm 2$   | $0.238 \pm 0.001$        |
|     | $0.097 \pm 0.003$ | $156 \pm 4$  | $0.239 \pm 0.001$        |
| 60  | $0.174 \pm 0.004$ | $450 \pm 10$ | $0.224 \pm 0.001$        |
|     | $0.176 \pm 0.006$ | $452 \pm 15$ | $0.226 \pm 0.001$        |
|     | $0.30 \pm 0.01$   | $863 \pm 26$ | $0.234 \pm 0.001$        |

Table ST2: Fit parameters  $a$  and  $b$ , along with the coefficient  $\alpha$ , obtained from non-linear fits of the density profiles for different groups  $N$ . Each  $N$  group includes three experimental realizations. Uncertainties represent standard deviation from the fitting procedure. Since  $b \gg \alpha$ , it follows that  $f_{\text{eff}}(r) \approx 0$  for small distances  $r$ .

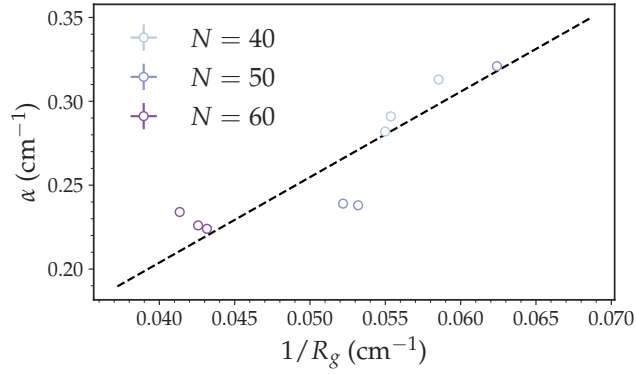

Figure SF3: Linear regression of the parameter  $\alpha$  as a function of the inverse radius of gyration ( $1/R_g$ ), with the intercept constrained to zero. The resulting fit yields a slope of  $5.10 \pm 0.01$  and a coefficient of determination  $R^2 = 0.8$ , indicating a proportional relationship between  $\alpha$  and  $1/R_g$ . Error bars are included for each data point but are too small to be visually distinguished on the scale of the plot.

#### SM-IV. INDUCED FORCES IN POLAR COORDINATES

Given a central force acting on a particle,

$$\vec{f}(r) = -f(r)\hat{r}, \quad (\text{SE4})$$

where  $\hat{r} = \vec{r}/r$ , Newton's second law in Cartesian coordinates can be written as  $\vec{\dot{v}} = \vec{f}$ , assuming unit mass for simplicity. When transforming to polar coordinates with velocity expressed as  $\vec{v} = (v \cos \theta, v \sin \theta)$ , the differential equations governing  $v$  and  $\theta$  acquire terms related to  $\vec{f}(r)$  of the form

$$\dot{v} = \frac{d}{dt} \left( \sqrt{v_x^2 + v_y^2} \right) = \frac{v_x \dot{v}_x + v_y \dot{v}_y}{v} = \frac{v_x f(r)(-\hat{r}_x) + v_y f(r)(-\hat{r}_y)}{v} = f(r)(-\hat{v} \cdot \hat{r}), \quad (\text{SE5})$$

and

$$\dot{\theta} = \frac{d}{dt} \left( \arctan \frac{v_y}{v_x} \right) = \frac{v_x \dot{v}_y - v_y \dot{v}_x}{v_x^2 + v_y^2} = \frac{v_x f(r)(-\hat{r}_y) - v_y f(r)(-\hat{r}_x)}{v^2} = f(r) \frac{1}{v} (-\hat{v} \times \hat{r}). \quad (\text{SE6})$$

From these expression, we obtain the terms  $F_{\text{eff}}^v$  and  $F_{\text{eff}}^\theta$  present in Eq. (6) of the main paper in the form

$$F_{\text{eff}}^v = A(-\hat{v} \cdot \hat{r}) f_{\text{eff}}(r), \quad F_{\text{eff}}^\theta = A \frac{1}{v} (-\hat{v} \times \hat{r}) f_{\text{eff}}(r). \quad (\text{SE7})$$

#### SM-V. STOCHASTIC MODEL INFERENCE FOR MOVEMENT IN THE CM REFERENCE FRAME

The Kramers-Moyal expansion [7] facilitates the transformation of a master equation into a Fokker-Planck equation for a stochastic variable  $y(t)$  of the form

$$\frac{\partial P(y, t)}{\partial t} = -\frac{\partial}{\partial y} [F(y)P(y, t)] + \frac{\partial^2}{\partial y^2} [G(y)P(y, t)], \quad (\text{SE8})$$

from which the corresponding Langevin equation can be derived as

$$\frac{dy(t)}{dt} = F(y, t) + \sqrt{2G(y, t)}\xi(t), \quad (\text{SE9})$$

where  $\xi(t)$  is an uncorrelated Gaussian noise. The Kramers-Moyal coefficients  $F(y, t)$  and  $G(y, t)$  (the drift and diffusion terms) are statistically defined as

$$\begin{aligned} F(x, t) &= \lim_{\tau \rightarrow 0} \frac{1}{\tau} \langle [y(t+\tau) - y(t)] | y(t) = x \rangle \\ G(x, t) &= \lim_{\tau \rightarrow 0} \frac{1}{2\tau} \langle [y(t+\tau) - y(t)]^2 | y(t) = x \rangle. \end{aligned} \quad (\text{SE10})$$

When we have a time series  $y_t$  and assume that the Kramers-Moyal coefficients are time-independent, these coefficients can be numerically estimated via a kernel-based regression of the form [8]:

$$\begin{aligned} F(x, \tau, h) &= \frac{1}{\tau} \left\langle \frac{K_h(x - y_t)}{\langle K_h(x - y_{t'}) \rangle_{t'}} (y_{t+\tau} - y_t) \right\rangle_t \\ G(x, \tau, h) &= \frac{1}{2\tau} \left\langle \frac{K_h(x - y_t)}{\langle K_h(y - y_{t'}) \rangle_{t'}} (y_{t+\tau} - y_t)^2 \right\rangle_t \end{aligned} \quad (\text{SE11})$$

where  $K_h(z) = h^{-1}\kappa(z/h)$  and  $\kappa(z)$  is the Epanechnikov kernel [9]

$$\kappa(z) = \begin{cases} \frac{3}{4\sqrt{5}} \left(1 - \frac{z^2}{5}\right) & \text{if } z^2 < 5 \\ 0 & \text{if } z^2 > 5 \end{cases}. \quad (\text{SE12})$$

The estimators obtained from the previous equations explicitly depend on both the time delay parameter  $\tau$  and the bandwidth value  $h$ . Since we analyze two independent stochastic functions  $\omega$  and  $v$ , each will have its own optimal  $\tau$  and  $h$  values. For the case of  $\omega$ , we find that  $\tau^* = 0.10\text{s}$  is sufficient to reduce correlations to nearly zero; for the speed  $v$ , a time delay of  $\tau^* = 0.04\text{s}$  was chosen. Given these  $\tau^*$  values, we select the bandwidth  $h$  using the algorithm introduced in Ref. [8]. Specifically, for each candidate  $h$ , we estimate  $F(x, \tau^*h)$  and  $G(x, \tau^*h)$ , generate synthetic time series for  $\omega$  and  $v$  by numerically integrating the corresponding Langevin equations with the estimated coefficients, and then re-infer the drift and diffusion coefficients  $\hat{F}(x, \tau^*, h)$  and  $\hat{G}(x, \tau^*, h)$  from these synthetic data. Finally, we compare the re-inferred drift and diffusion to those estimated directly from the original time series,

$$\xi(h) = \frac{\int |f(x, \tau^*h) - \hat{f}(x, \tau^*h)| \sqrt{\pi(x)\hat{\pi}(x)} dy}{\int \sqrt{\pi(x)\hat{\pi}(x)} dx}, \quad (\text{SE13})$$

averaging over 1000 independent synthetic time series. In Eq. (SE13),  $f$  can be either  $F$  or  $D$ ;  $\pi(x)$  denotes the steady-state distribution obtained from  $f$ , while  $\hat{\pi}(x)$  is derived from  $\hat{f}$ . The optimal bandwidth  $h^*$  is chosen as the value of the first local minimum of the function  $\xi(h)$ . The trivial minimum corresponding to  $h \rightarrow \infty$  is discarded to prevent the trivial solution of constant  $F$  and  $G$ .

To focus on free movement unaffected by the trapping potential, only trajectory segments within  $r < R_g$  are analyzed. Furthermore, we assume that all fish exhibit equivalent dynamics, enabling the aggregation of data across all individuals to enhance statistical robustness. For  $\omega$ , the optimal bandwidth is  $h^* \sim 0.11$  for both drift and diffusion coefficients. For the speed  $v$ , the optimal bandwidth is  $h^* = 0.8$  for the drift term and  $h^* = 0.53$  for the diffusion term (see Fig. SF4).

The results of applying this method to the speed and turning rate are shown in Fig. SF5. The computed drift and diffusion coefficients are consistent across different group sizes, with the behavior of  $\omega$ —the turning rate—being nearly identical in all groups. This finding aligns with the collapse of the turning rate distribution shown in Fig. SF14 and suggests that the observed dynamics are primarily governed by intrinsic properties of the individual fish, rather than collective effects.

We approximate the resulting coefficients by fitting them to simple reasonable functions, namely

$$\begin{aligned} f_v(v) &= \frac{\gamma_1}{v} - \gamma_2 v, \\ g_v(v) &= \delta_1 v + \delta_2, \\ f_\omega(\omega) &= -\kappa\omega, \\ g_\omega(\omega) &= n_1|\omega| + n_2. \end{aligned} \quad (\text{SE14})$$

Table ST3 summarizes the values of the parameters obtained through non-linear fitting.

Although the fitted functions may appear somewhat arbitrary, they possess meaningful physical interpretations. For the velocity drift term  $f_v(v)$ , the second term represents a drag force, modeled as a linear friction with coefficient  $\gamma_2$ . This is appropriate for small fish like black neon tetras, which operate at low Reynolds numbers ( $\lesssim 1000$ ) [10]. The first term accounts for the positive definiteness of speed, preventing it from approaching zero by providing an acceleration mechanism that sustains movement. Indeed, this drift term can be interpreted as an active friction force of the form  $f_v(v) = -\gamma_2 \frac{v^2 - v_0^2}{v}$ , where  $v_0 = \sqrt{\gamma_1/\gamma_2}$  represents a characteristic speed  $v_0$  for fish motion in the CM reference frame. Similar non-linear mechanisms have been observed in Brownian particles far from equilibrium, especially in systems where particles are powered by an internal energy depot [11]. The diffusion term  $g_v(v)$  exhibits a linear dependence on speed, with an additional constant parameter  $\delta_2 \neq 0$ , ensuring that the system does not have an

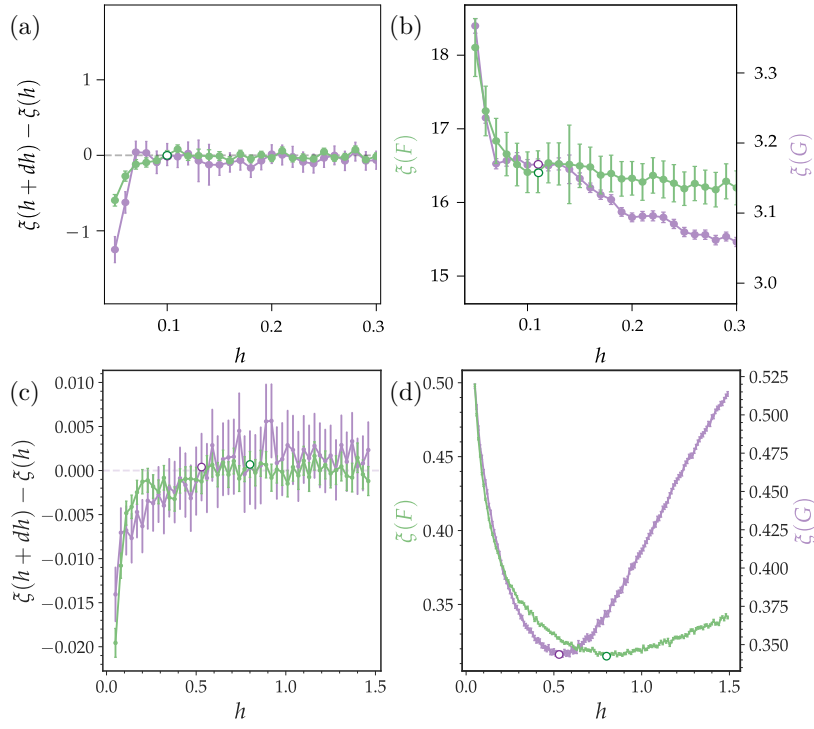

Figure SF4: Optimization of the bandwidth  $h$  for the turning speed  $\omega$  and velocity  $v$ . (a) shows the difference between two consecutive values of  $\xi(h)$ ; when this difference approaches zero, the corresponding  $h^*$  is considered the optimal value. (b) displays the  $\xi(h)$  function itself, with the optimal  $h^*$  chosen as the first minimum, indicated by a white point. (c), (d) Similar optimization of the bandwidth for the velocity  $v$  of fish. Although the figure presented is based on data from the group with  $N = 60$ , comparable results were obtained for the other group sizes.

| $N$ | $F_v(v)$                                          |                                          | $G_v(v)$                                  |                                                     |
|-----|---------------------------------------------------|------------------------------------------|-------------------------------------------|-----------------------------------------------------|
| 40  | $\gamma_1 = 3.14 \pm 0.01 \text{cm}^2/\text{s}^3$ | $\gamma_2 = 0.20 \pm 0.01 \text{s}^{-1}$ | $\delta_1 = 0.20 \pm 0.01 \text{s}^{1/2}$ | $\delta_2 = 2.23 \pm 0.02 \text{cm}/\text{s}^{3/2}$ |
| 50  | $\gamma_1 = 3.93 \pm 0.01 \text{cm}^2/\text{s}^3$ | $\gamma_2 = 0.20 \pm 0.01 \text{s}^{-1}$ | $\delta_1 = 0.22 \pm 0.01 \text{s}^{1/2}$ | $\delta_2 = 2.44 \pm 0.02 \text{cm}/\text{s}^{3/2}$ |
| 60  | $\gamma_1 = 4.15 \pm 0.01 \text{cm}^2/\text{s}^3$ | $\gamma_2 = 0.20 \pm 0.01 \text{s}^{-1}$ | $\delta_1 = 0.19 \pm 0.01 \text{s}^{1/2}$ | $\delta_2 = 2.45 \pm 0.03 \text{cm}/\text{s}^{3/2}$ |

| $N$ | $F_\omega(\omega)$                     | $G_\omega(\omega)$                   |                                            |
|-----|----------------------------------------|--------------------------------------|--------------------------------------------|
| 40  | $\kappa = 9.92 \pm 0.01 \text{s}^{-1}$ | $n_1 = 3.03 \pm 0.02 \text{s}^{1/2}$ | $n_2 = 12 \pm 1 \text{rad}/\text{s}^{3/2}$ |
| 50  | $\kappa = 9.92 \pm 0.02 \text{s}^{-1}$ | $n_1 = 3.02 \pm 0.02 \text{s}^{1/2}$ | $n_2 = 13 \pm 2 \text{rad}/\text{s}^{3/2}$ |
| 60  | $\kappa = 9.91 \pm 0.01 \text{s}^{-1}$ | $n_1 = 3.02 \pm 0.02 \text{s}^{1/2}$ | $n_2 = 13 \pm 2 \text{rad}/\text{s}^{3/2}$ |

Table ST3: Parameters obtained from fitting drift and diffusion terms.

absorbing state. Although in a different context, a similar inference of Langevin equations in a study of amoeboid social motion revealed a noise term with a linear dependence on speed [12].

The drift term  $f_\omega(\omega)$  also exhibits a simple linear drag-like form, reflecting a tendency to maintain the previous heading direction. The diffusion term  $g_\omega(\omega)$  is symmetric around  $\omega = 0$  and has a positive minimum value, which prevents  $\omega$  from reaching an absorbing state.

Finally, the last free parameter,  $A$ , is determined by minimizing the mean squared error (MSE) between the radial density  $\rho$  obtained from experimental data,  $\rho^{\text{exp}}$ , and that computed from simulations,  $\rho^{\text{sim}}$ . The MSE is defined as

$$\text{MSE} = \frac{1}{q} \sum_{n=1}^q \left( \rho_q^{\text{exp}} - \rho_q^{\text{sim}} \right)^2,$$

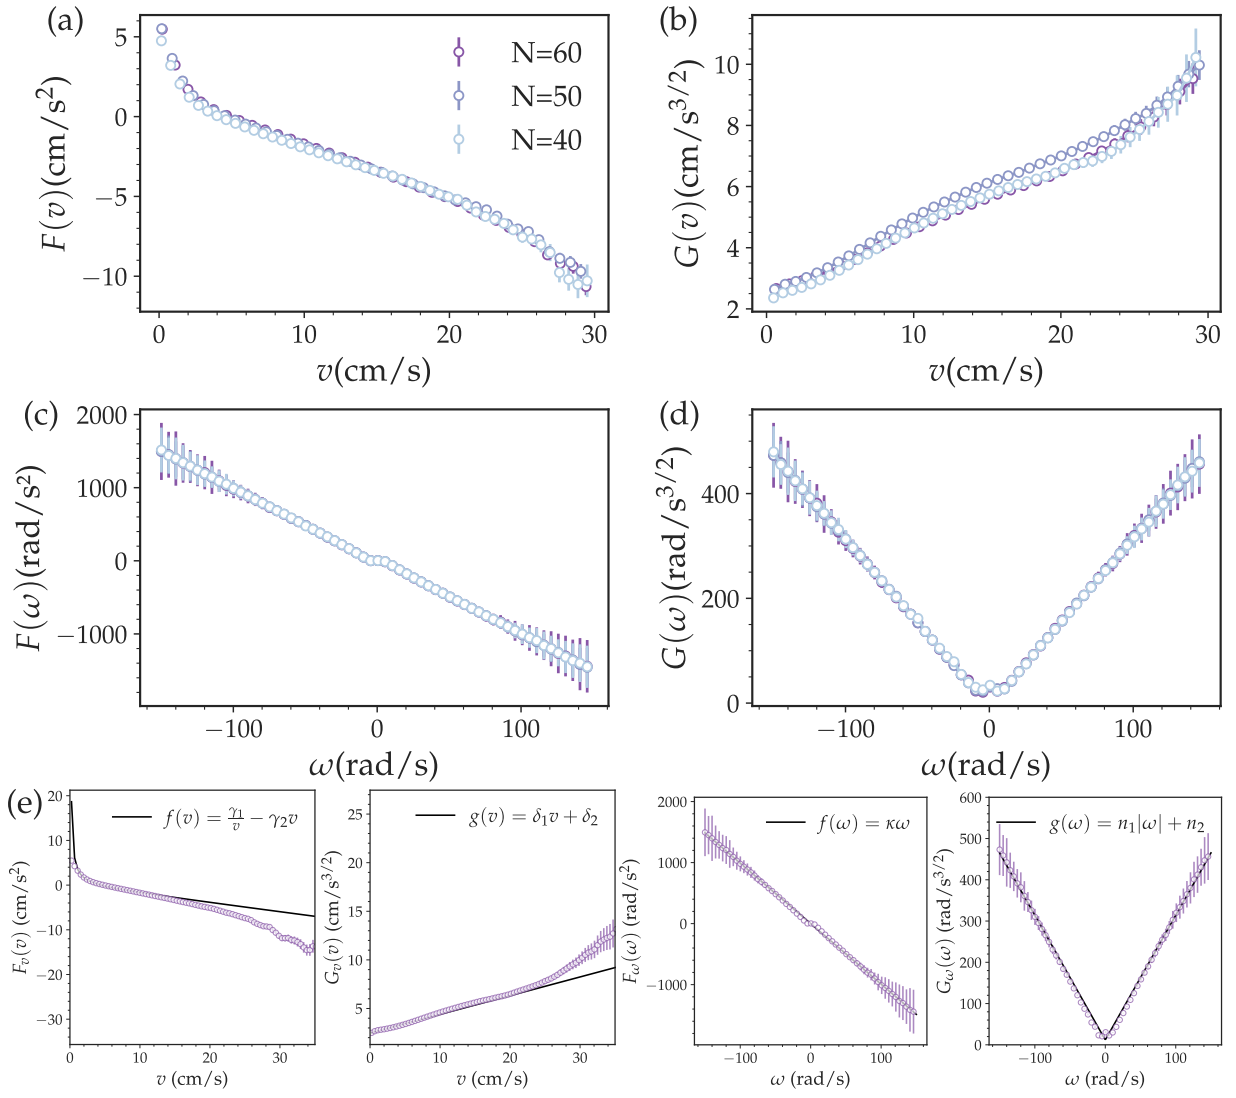

Figure SF5: (a), (c) Deterministic and (b), (d) stochastic contributions to individual fish speed and turning rate. All these contributions have been estimated using a kernel-based regression method. All terms include error bars representing the standard error (the standard deviation divided by the square root of the number of samples). (e) Example of the fit for  $N = 60$  showing the different terms: the drift and diffusion coefficients for speed and turning rate, respectively. During the fitting process, data points with higher statistical significance—corresponding to lower speeds and turning rates near zero—were assigned higher weights. The quality of the fits was evaluated using the coefficient of determination, with  $r^2 = 0.95$  for the drift term of the speed equation and  $r^2 > 0.99$  for all other terms within the data range considered.



where  $q$  denotes the number of radial bins used to compute the radial density. The numerical radial density is averaged over 30 independent realizations, providing sufficient statistical accuracy for comparison with experimental data while remaining computationally efficient. The parameter  $A$  exhibits only weak variation across experiments with different group sizes  $N$ ; therefore, we select a single representative value by minimizing the mean squared error for a realization with  $N = 60$ . We then verify that this value yields similarly good agreement for the other two group sizes. The resulting estimate is  $A = 30.6 \pm 0.4 \text{ cm}^2 \text{ s}^{-2}$ . This approach is motivated by the fact that  $\rho$  is the observable most sensitive to variations in  $A$ .

## SM-VI. SYNTHETIC SCHOOLS

Using the model developed to describe the dynamics of relative movement in the CM reference frame and the movement of the CM as a pseudo-particle, synthetic schools of size  $N$  can be generated via Eq. (1) in the main paper, namely

$$\vec{r}_i^{\text{lab}}(t) = \vec{R}(t) + \vec{r}_i(t), \quad (\text{SE15})$$

where the position of the CM,  $\vec{R}(t)$ , is obtained from Eq. (2), and the  $N$  (independent) relative trajectories in the CM reference frame,  $\vec{r}_i(t)$ , are obtained by integrating Eq. (6). Since the  $N$  relative trajectories are uncorrelated, the resulting synthetic schools are expected to reproduce the global properties of a real school, or individual fish behavior, but may fail to capture observables related to correlations among fish, such as the relative distance to nearest neighbors [13].

## SM-VII. INFINITE LIMIT OF SYNTHETIC SCHOOLS

In the limit  $N \rightarrow \infty$ , the radius of gyration also tends to infinity,  $R_g \rightarrow \infty$ , which necessarily means that the space cannot be confined—that is, the tank walls would effectively be located at infinity. This leads to an equation of motion for the center of mass in which the hard-wall force  $\vec{F}(\vec{R})$  vanishes, and the equations governing the relative motion of individual fish in the CM frame exclude the effective forces  $F_{\text{eff}}^v$  and  $F_{\text{eff}}^\theta$ . In this limit, the equations of motion of the CM read

$$\frac{d\vec{R}}{dt} = \vec{V}, \quad \frac{d\vec{V}}{dt} = -\gamma_0 (V - V_0) \frac{\vec{V}}{V} + \sqrt{2D}\xi(t), \quad (\text{SE16})$$

while the equations for the relative motion in the CM frame have the form

$$\begin{aligned} \dot{x} &= v \cos \theta, \\ \dot{y} &= v \sin \theta, \\ \dot{v} &= f_v(v) + g_v(v) \xi_v(t), \quad , \\ \dot{\theta} &= \omega, \\ \dot{\omega} &= f_\omega(\omega) + g_\omega(\omega) \xi_\omega(t) \end{aligned} \quad (\text{SE17})$$

The Langevin Eqs. (SE16) have been extensively studied in the literature [11, 14], and it has been shown that, in the long-time limit, the stationary velocity distribution takes the form, in Cartesian coordinates [11, 14]:

$$P_0(\vec{V}) = \mathcal{N} \exp \left\{ -\frac{\gamma_0}{2D} (|\vec{V}| - V_0)^2 \right\}, \quad (\text{SE18})$$

where  $\mathcal{N}$  represents a normalization constant. Thus, for the modulus of the velocity, we have

$$P_0(V) = \mathcal{N} V \exp \left\{ -\frac{\gamma_0}{2D} (V - V_0)^2 \right\}. \quad (\text{SE19})$$

For the relative movement equations, Eqs. (SE17), we can derive the probability density function (PDF)  $P(v, \omega)$  analytically, given the fitted functions in Eq. (SE14). Since  $\omega$  and  $v$  are independent variables, the joint PDF factorizes as  $P(v, \omega) = P(v)P(\omega)$ .

The stationary solutions for  $P(v)$  and  $P(\omega)$  are obtained from their respective Fokker-Planck equations, which, for a single variable, take the form [15]:

$$\partial_t P(y, t) = -\partial_y (f(y)P(y, t)) + \frac{1}{2} \partial_y^2 (g(y)^2 P(y, t)), \quad (\text{SE20})$$



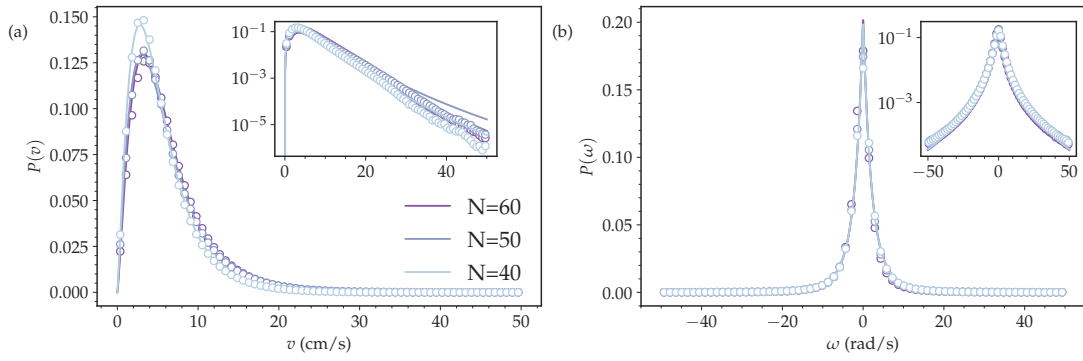

Figure SF6: (a) and (b) Probability density functions for the speed and turning rate of freely swimming fish derived from experimental data (points) are compared with the analytical predictions obtained from the fitted drift and diffusion coefficients (solid line).

where  $y$  corresponds to either  $v$  or  $\omega$ .

The stationary solution of the Fokker-Planck equation Eq. (SE20) with reflecting boundary conditions is [15]

$$P_0(y) = \frac{\mathcal{N}}{g(y)^2} \exp \left[ 2 \int_{-\infty}^y dz \frac{f(z)}{g(z)^2} \right], \quad (\text{SE21})$$

and using the drift and diffusion coefficients previously fitted for the velocity  $v$ , we obtain

$$P_0(v) = \mathcal{N} \frac{v^{2\gamma_1/\delta_2^2}}{(\delta_1 v + \delta_2)^{2(\beta_+ + 1)}} \exp \left\{ 2\delta_2 \frac{\beta_-}{(\delta_1 v + \delta_2)} \right\}; \quad \beta_{\pm} = (\gamma_1/\delta_2^2 \pm \gamma_2/\delta_1^2). \quad (\text{SE22})$$

Similarly, for the turning rate  $\omega$  the solution reads

$$P_0(\omega) = \frac{\mathcal{N}}{(n_1 |\omega| + n_2)^{2(1+\kappa/n_1^2)}} \exp \left\{ -\frac{2\kappa n_2}{n_1^2 (n_2 + n_1 |\omega|)} \right\}. \quad (\text{SE23})$$

Figure SF6 compares the analytical PDFs in Eqs. (SE22) and (SE23) with the empirical distributions of velocity  $v$  and turning rate  $\omega$ , respectively, obtained from the empirical data in trajectories restricted to the region  $r < R_g$ . The parameters  $\gamma_i$ ,  $\delta_i$ ,  $n_i$  and  $\kappa$  used are from Table ST3. As seen, the analytical solutions match the empirical data very well, with the exception of the tail of the velocity distribution at large  $v$ , as highlighted in the inset of Fig. SF6(a). This discrepancy may be due to a slight curvature in the diffusion term (Fig. SF5(b)) that is not captured by the linear approximation  $g_v(v) = \delta_1 v + \delta_2$ . A similar expression for the speed PDF, given in Eq. (SE22), has been identified in the study of social amoebae, where it features both a power-law component and an exponential tail [12].

## SM-VIII. COMPARISON BETWEEN EXPERIMENTAL AND FINITE SYNTHETIC SCHOOLS

By simulating a synthetic school of finite size  $N$ , we can compare its properties with those of our experimental schools. As an illustration, Fig. SF7 presents a side-by-side comparison of a real fish trajectory and one generated by the model. The trajectories display remarkably similar motion patterns, highlighting the model's capability to replicate naturalistic behavior.

Regarding individual properties, our model effectively captures the burst-and-coast swimming strategy exhibited by black neon tetra and many other fish species [16]. This pattern consists of alternating phases of rapid acceleration (bursts) and passive gliding (coasts). Importantly, these speed oscillations often exhibit a degree of synchronization among individuals: a burst by one fish can trigger similar accelerations in others. This phenomenon has been previously investigated in pairwise interactions [17], group contexts [18], and even modeled using neural networks frameworks [10]. As shown in Fig. SF8, synchronized speed oscillations emerge naturally within our modeling framework.

Since the model describes a group of random walkers, it is appropriate to characterize their dynamics using the mean square displacement (MSD) as a function of time [15]. The MSD in the laboratory frame is defined as the average squared displacement of individual fish at time  $t$ , namely

$$\delta \vec{r}^{\text{lab}^2}(t) = \frac{1}{T-t} \frac{1}{N} \sum_{t_0=0}^{T-t-1} \sum_{i=1}^N \left[ \vec{r}_i^{\text{lab}}(t_0+t) - \vec{r}_i^{\text{lab}}(t_0) \right]^2, \quad (\text{SE24})$$

where  $\vec{r}_i^{\text{lab}}(t)$  indicates the position of an individual at time  $t$ , and where we have averaged over the ensemble and over all time lags of duration  $t$  in the interval  $[0, T]$ . This definition of MSD is consistent with that used in [19] to measure diffusion in starling flocks, both in the laboratory frame and in the center-of-mass reference frame.

Using this definition, we computed the MSD from both experimental trajectories and simulated data, as shown in Fig. SF9. In the laboratory frame, the MSD exhibits an oscillatory behavior, especially evident in the plateau region. This oscillation reflects the coherent movement of the entire group, which moves in looping trajectories constrained by the tank boundaries. Our model successfully reproduces these oscillations, showing good agreement, particularly for the group of size  $N = 60$ . For smaller groups, the experimental MSD exhibits greater variability due to fluctuations, and although the model does not precisely replicate each realization, it consistently captures the overall intermediate trend observed across the diverse experimental outcomes.

Beyond individual dynamics, the model also successfully captures key collective observables typically used to characterize fish schools. One such observable is polarization, which quantifies the degree of alignment in the velocities of individuals within a group. Defined as

$$\phi = \left| \frac{1}{N} \sum \frac{\vec{v}_i^{\text{lab}}}{v_i^{\text{lab}}} \right|, \quad (\text{SE25})$$

Polarization has been widely studied in the context of collective motion to characterize the order within groups of moving animals [20]. In Fig. SF10(a), we present the empirical distribution of polarization, averaged across all experiments for each school size. While there is a pronounced peak near  $\phi \approx 1$ , indicating a strong tendency for directional order among black neon tetras, the distribution also demonstrates a notable flexibility to adopt disordered configurations. This is evidenced by the exponential tail for small  $\phi$  in the PDF, as shown in Fig. SF10(a). Remarkably, our model captures this variability, producing a distribution that closely aligns with the experimental observations.

Finally, we examine the tendency of fish to remain at the periphery of the group [21]. By defining an individual as being on the periphery of the school if it belongs to the convex hull of the group at a given frame, we can compute the distribution of the time  $\Delta t_{\text{border}}$  that a fish spends on the periphery before leaving it (i.e., the interval between entering and exiting the convex hull) [21]. As shown in Fig. SF10(b), the model accurately reproduces the empirical distribution, indicating that the tendency to avoid the group's border is a trait embedded in the individual fish dynamics.

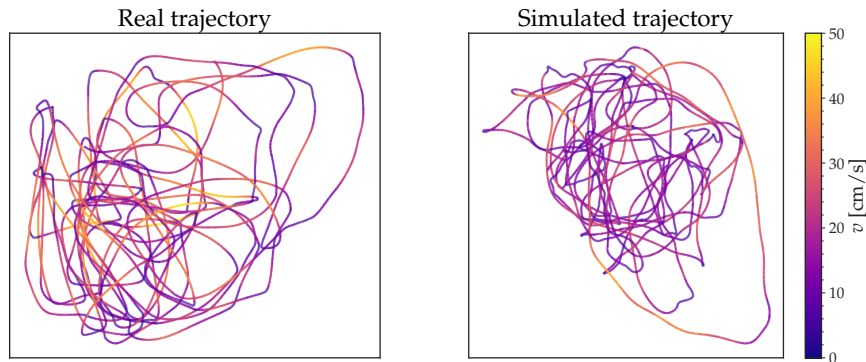

Figure SF7: Comparison between a real individual fish trajectory and a corresponding simulated trajectory of the same duration. Both trajectories pertain to a group size  $N = 60$ .

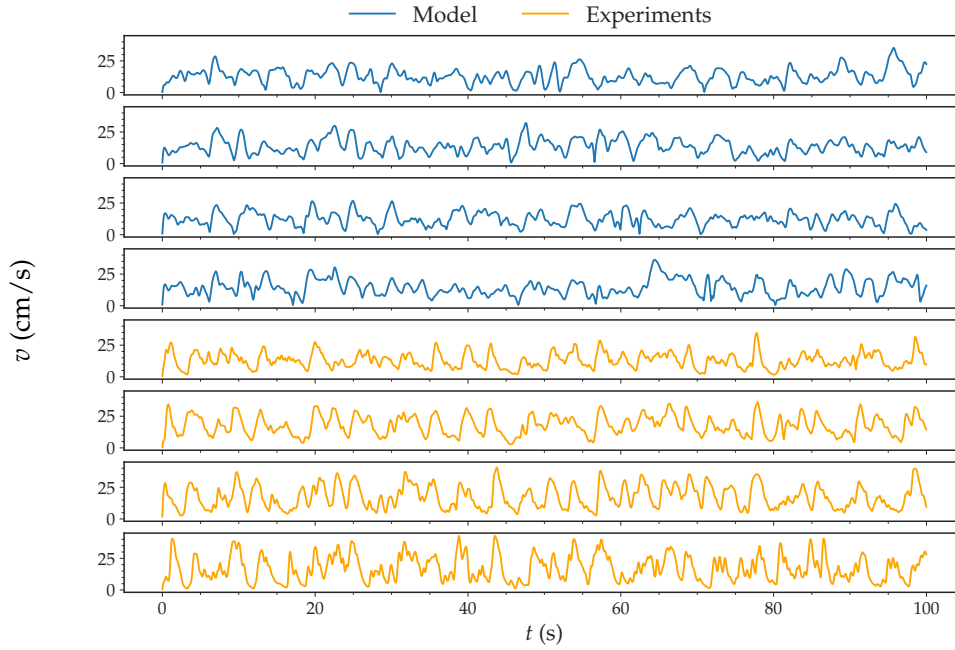

Figure SF8: Temporal evolution of speed for different fish in both the model and experimental data demonstrates the model's ability to reproduce synchronization phenomena. To enable direct comparison, the Gaussian filter used for experimental data have also been applied to simulation data.

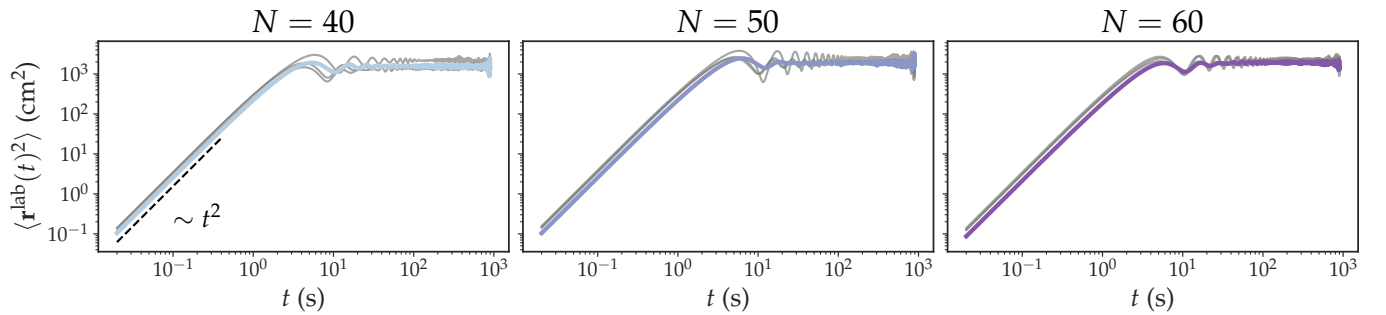

Figure SF9: Mean square displacement (MSD) in the laboratory frame for group sizes  $N = 40, 50$ , and  $60$ . Gray lines represent individual experimental realizations, while colored lines depict the corresponding model predictions. The MSD displays a ballistic regime at short times followed by saturation at long times due to confinement within the tank. The subtle oscillations observed in the plateau region are indicative of the collective motion of the group's center of mass as it circulates inside the tank.

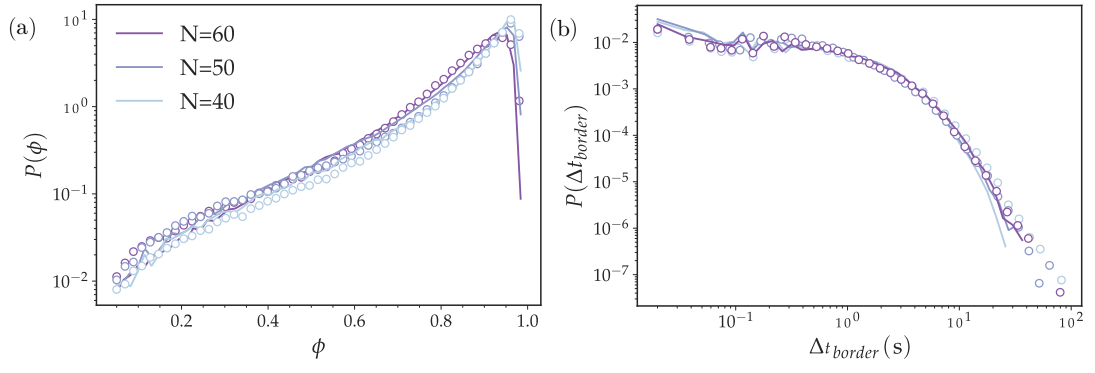

Figure SF10: (a) Probability density functions (PDF) of polarization for experimental data (points) compared with simulation results (solid line). (b) PDF of the time a fish spends on the border of the convex hull, with experimental data (points) and simulation results (solid line).

## SM-IX. SUPPLEMENTAL FIGURES

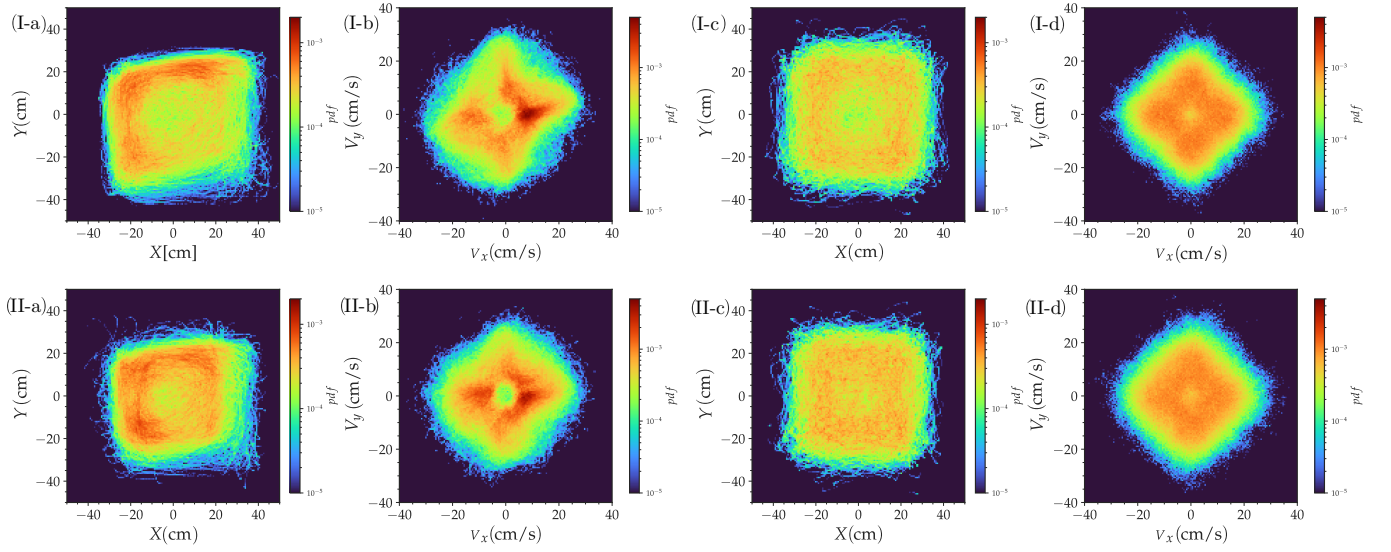

Figure SF11: Center-of-mass dynamics for two group sizes. The number in each subplot label indicates the group size: (I) corresponds to  $N = 50$ , and (II) to  $N = 40$ . The letters denote the type of data: (a), (b) represent experimental position and velocity distributions, respectively, while (c), (d) show the corresponding simulation results. Each row displays the full set of observables for a given group size, enabling direct comparisons between experimental data and model simulations. For the experimental data, each probability density function (PDF) is obtained by aggregating over three independent experiments. For the simulations, the PDFs are derived from three independent runs of equal duration to the experiments, performed using the mean parameter values reported in Table ST1.

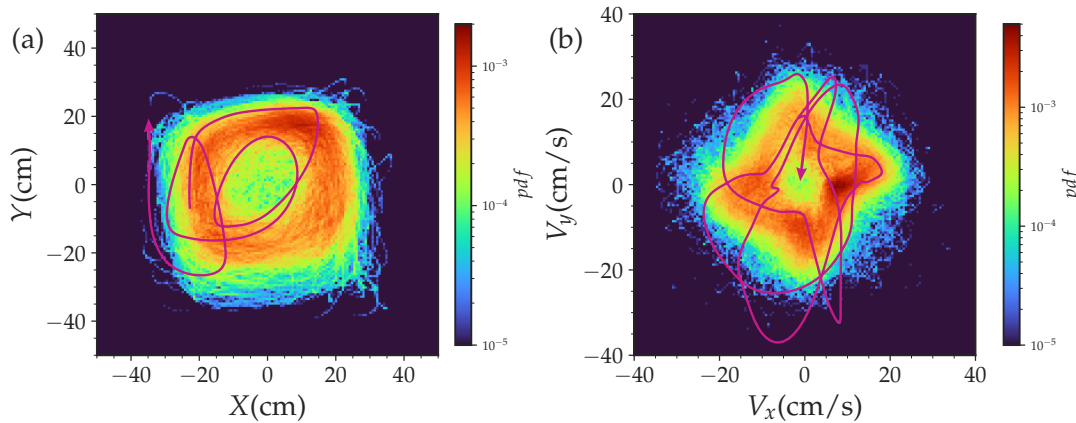

Figure SF12: Probability density functions (PDFs) of the center-of-mass position (right) and velocity (left) obtained from three experiments with group size  $N = 60$ . The pink line shows a representative segment of the CM trajectory, with the arrow indicating the direction of motion at the final frame. The trajectory demonstrates a tendency to slide along the tank walls, although the motion does not necessarily follow a simple loop around tank walls.

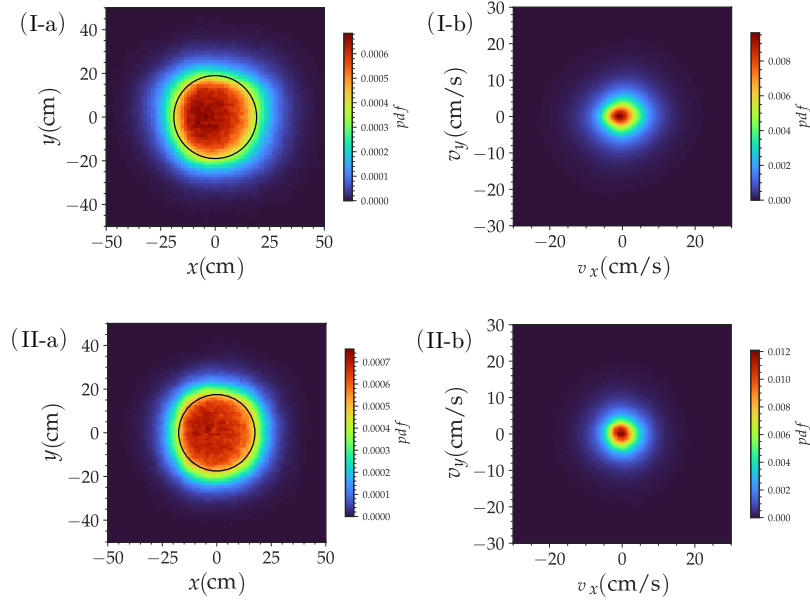

Figure SF13: Fish in the center-of-mass reference frame: (a) positions derived from the PDF aggregating three experimental realizations for two different group sizes: (I) ( $N=50$ ) and (II) ( $N=40$ ). The schools exhibit approximately radial symmetry around the center of mass. The black circle indicates the mean radius of gyration for each group, highlighting the typical spatial extent of the school. (b) shows the distribution of individual velocity components within the same realizations.

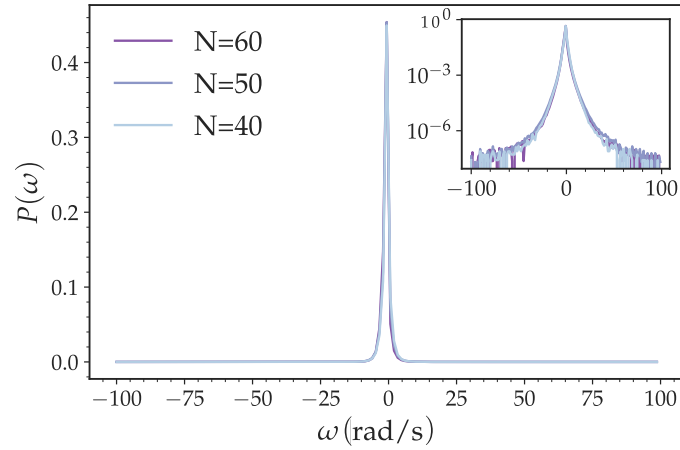

Figure SF14: Distribution of turning rate for groups of  $N = 40, 50$ , and  $60$  individuals. The collapse of these distributions across different group sizes emphasizes the universality of this observable.

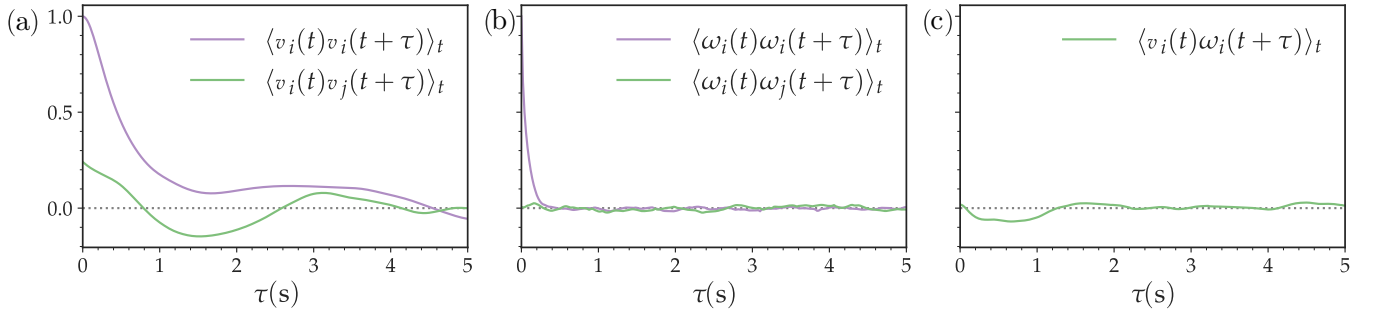

Figure SF15: Average temporal correlations computed from experimental data. Panel (a) shows the autocorrelation of speed  $v$  for individual fish and the cross-correlation of speed between fish pairs; panel (b) displays the same for angular rate  $\omega$ ; and panel (c) presents the cross-correlation between speed and angular rate for the same individual. All cross-correlations are computed over time lags  $\tau$  and averaged over 80 randomly selected individual pairs from a group of 60 fish. Correlations involving the same individual are computed using data from 80 fish within the same group but at different initial times.

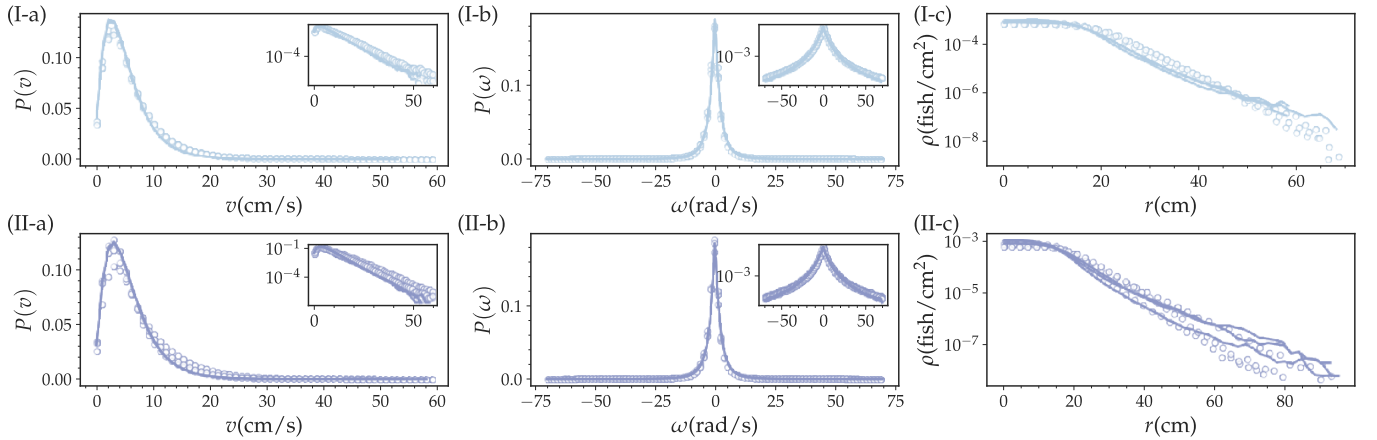

Figure SF16: Statistical properties of collective motion in the center-of-mass reference frame for two group sizes. Roman numerals denote the group size: *I* corresponds to  $N = 40$ , and *II* to  $N = 50$ . Panels (a) and (b) show the distribution of individual speed  $v$  and turning rate  $\omega$ , respectively, with points representing experimental data and solid lines indicating simulation results. Inset figures display these distributions on a logarithmic scale. Panels (c) display the radial density distribution, following the same convention: points for experimental data and solid lines for simulations.



- [1] E. Gimeno, V. Quera, F. S. Beltran, and R. Dolado, Differences in shoaling behavior in two species of freshwater fish (*Danio rerio* and *Hyphessobrycon herbertaxelrodi*)., *Journal of Comparative Psychology* **130**, 358 (2016).
- [2] F. Romero-Ferrero, M. G. Bergomi, R. C. Hinz, F. J. H. Heras, and G. G. de Polavieja, Idtracker.ai: Tracking all individuals in small or large collectives of unmarked animals, *Nature Methods* **16**, 179 (2019).
- [3] M. S. Nixon and A. S. Aguado, *Feature Extraction and Image Processing*, 2nd ed. (Acad. Press, Amsterdam, 2010).
- [4] P. Virtanen, R. Gommers, T. E. Oliphant, M. Haberland, T. Reddy, D. Cournapeau, E. Burovski, P. Peterson, W. Weckesser, J. Bright, S. J. van der Walt, M. Brett, J. Wilson, K. J. Millman, N. Mayorov, A. R. J. Nelson, E. Jones, R. Kern, E. Larson, C. J. Carey, Í. Polat, Y. Feng, E. W. Moore, J. VanderPlas, D. Laxalde, J. Perktold, R. Cimrman, I. Henriksen, E. A. Quintero, C. R. Harris, A. M. Archibald, A. H. Ribeiro, F. Pedregosa, and P. van Mulbregt, SciPy 1.0: Fundamental algorithms for scientific computing in Python, *Nature Methods* **17**, 261 (2020).
- [5] K. P. Burnham and D. R. Anderson, *Model Selection and Multimodel Inference: A Practical Information-Theoretic Approach*, 2nd ed. (Springer, New York, 2002).
- [6] E. Shaw, Schooling fishes: The school, a truly egalitarian form of organization in which all members of the group are alike in influence, offers substantial benefits to its participants, *American Scientist* **66**, 166 (1978).
- [7] H. Risken, *The Fokker-Planck Equation: Methods of Solution and Applications*, edited by H. Haken, Springer Series in Synergetics, Vol. 18 (Springer, Berlin, Heidelberg, 1996).
- [8] D. Lamouroux and K. Lehnertz, Kernel-based regression of drift and diffusion coefficients of stochastic processes, *Physics Letters A* **373**, 3507 (2009).
- [9] V. A. Epanechnikov, Non-parametric estimation of a multivariate probability density, *Theory of Probability & Its Applications* **14**, 153 (1969), <https://doi.org/10.1137/1114019>.
- [10] L. Gyllingberg, A. Szorkovszky, and D. J. T. Sumpter, Using neuronal models to capture burst-and-glide motion and leadership in fish, *Journal of The Royal Society Interface* **20**, 20230212 (2023).
- [11] U. Erdmann, W. Ebeling, L. Schimansky-Geier, and F. Schweitzer, Brownian particles far from equilibrium, *The European Physical Journal B - Condensed Matter and Complex Systems* **15**, 105 (2000), [cond-mat/9912465](https://doi.org/10.1007/s001470000246).
- [12] H. U. Bödeker, C. Beta, T. D. Frank, and E. Bodenschatz, Quantitative analysis of random ameboid motion, *EPL (Europhysics Letters)* **90**, 28005 (2010).
- [13] Y. Katz, K. Tunstrom, C. C. Ioannou, C. Huepe, and I. D. Couzin, Inferring the structure and dynamics of interactions in schooling fish, *Proceedings of the National Academy of Sciences* **108**, 18720 (2011).
- [14] P. Romanczuk, M. Bär, W. Ebeling, B. Lindner, and L. Schimansky-Geier, Active Brownian particles, *The European Physical Journal Special Topics* **202**, 1 (2012).
- [15] C. W. Gardiner, *Handbook of Stochastic Methods for Physics, Chemistry, and the Natural Sciences* (Springer-Verlag, 1985) google-Books-ID: cRfvAAAAMAAJ.
- [16] J. J. Videler and D. Weihs, Energetic advantages of burst-and-coast swimming of fish at high speeds, *Journal of Experimental Biology* **97**, 169 (1982).
- [17] D. S. Calovi, A. Litchinko, V. Lecheval, U. Lopez, A. Pérez Escudero, H. Chaté, C. Sire, and G. Theraulaz, Disentangling and modeling interactions in fish with burst-and-coast swimming reveal distinct alignment and attraction behaviors, *PLoS Computational Biology* **14**, e1005933 (2018).
- [18] R. Harpaz, G. Tkačik, and E. Schneidman, Discrete modes of social information processing predict individual behavior of fish in a group, *Proceedings of the National Academy of Sciences* **114**, 10149 (2017), publisher: Proceedings of the National Academy of Sciences.
- [19] A. Cavagna, S. M. D. Queirós, I. Giardina, F. Stefanini, and M. Viale, Diffusion of individual birds in starling flocks, *Proceedings of the Royal Society B: Biological Sciences* **280**, 20122484 (2013), publisher: Royal Society.
- [20] T. Vicsek, A. Czirók, E. Ben-Jacob, I. Cohen, and O. Shochet, Novel Type of Phase Transition in a System of Self-Driven Particles, *Physical Review Letters* **75**, 1226 (1995), publisher: American Physical Society.
- [21] A. Puy, E. Gimeno, F. S. Beltran, R. Dolado, M. C. Miguel, C. C. Ioannou, and R. Pastor-Satorras, *Perceived risk determines spatial position in fish shoals through altered rules of interaction* (2024), arXiv:2410.09264 [physics].
